# Supplementary material for: Statistically Guided Divide-and-Conquer for Sparse Factorization of Large Matrix
Source: arXiv:2003.07898 source file (2020-03-17)
Supplement: Supplementary file 1 [file table-supplement.tex]

\begin{table}[H]
  \caption{Results of Model II under different rank and SNR}\label{tab:model-1}
  \centering
  \resizebox{\columnwidth}{!}{
    \subfloat[SNR=0.25, $r=3$]{
    %\subcaptionbox{SNR=0.25, $r=3$}{
      \begin{tabular}{cccccc}
        \hline
        Method            & Er(C)$\times 10^3$ & Er(XC)$\times 10^3$ & FPR (\%) & FNR (\%) & Time (s) \\
        \hline
        \multicolumn{6}{c}{$p=100$}                                                                   \\
        RRR               & 29325.43           & 1125.52             & 100.00   & 0.00     & 0.10     \\
        ACS-seq           & 5.47               & 342.95              & 0.97     & 10.88    & 0.44     \\
        ACS-par (rrr)     & 5.85               & 358.02              & 2.88     & 12.67    & 7.03     \\
        ACS-par(lasso)    & 3.86               & 271.37              & 1.97     & 8.50     & 8.08     \\
        SRRR              & 6.04               & 531.47              & 61.30    & 0.00     & 6.31     \\
        SOFAR             & 66.94              & 6600.95             & 2.94     & 92.00    & 10.95    \\
        Stage-seq         & 3.33               & 208.52              & 0.83     & 9.23     & 0.49     \\
        Stage-par (lasso) & 3.22               & 230.20              & 1.01     & 9.54     & 1.11     \\
        Stage-par (rrr)   & 3.84               & 229.24              & 0.82     & 8.48     & 0.13     \\
        \hline
        \multicolumn{6}{c}{$p=200$}                                                                   \\
        RRR               & 23.60              & 1129.28             & 100.00   & 0.00     & 0.12     \\
        ACS-seq           & 3.05               & 373.80              & 0.67     & 11.33    & 1.51     \\
        ACS-par (rrr)     & 2.77               & 360.29              & 1.60     & 15.27    & 8.36     \\
        ACS-par(lasso)    & 2.29               & 315.43              & 1.46     & 9.02     & 9.03     \\
        SRRR              & 4.58               & 831.61              & 75.31    & 0.00     & 6.86     \\
        SOFAR             & 36.25              & 7302.63             & 0.00     & 100.00   & 12.65    \\
        Stage-seq         & 1.97               & 237.26              & 0.56     & 10.19    & 0.51     \\
        Stage-par (lasso) & 2.06               & 277.92              & 0.71     & 11.33    & 1.01     \\
        Stage-par (rrr)   & 2.25               & 265.47              & 0.56     & 9.83     & 0.18     \\
        \hline
        \multicolumn{6}{c}{$p=400$}                                                                   \\
        RRR               & 14.56              & 1105.04             & 100.00   & 0.00     & 0.44     \\
        ACS-seq           & 1.67               & 412.06              & 0.39     & 13.31    & 11.43    \\
        ACS-par (rrr)     & 1.51               & 375.35              & 0.93     & 13.50    & 13.08    \\
        ACS-par(lasso)    & 1.24               & 344.88              & 0.96     & 10.44    & 12.95    \\
        SRRR              & 2.27               & 967.05              & 54.06    & 0.00     & 21.17    \\
        SOFAR             & 18.13              & 7316.23             & 0.00     & 100.00   & 30.81    \\
        Stage-seq         & 1.07               & 260.14              & 0.33     & 11.96    & 1.12     \\
        Stage-par (lasso) & 1.13               & 310.70              & 0.42     & 11.85    & 1.42     \\
        Stage-par (rrr)   & 1.18               & 280.75              & 0.31     & 9.08     & 0.55     \\
        \hline
        % \multicolumn{6}{c}{Model-1, snr=0.25, r=3}                              \\
      \end{tabular}
    }
    \subfloat[SNR=0.25, $r=6$]{
    %\subcaptionbox{SNR=0.25, $r=6$}{
      \begin{tabular}{ccccc}
        \hline
        Er(C)$\times 10^3$ & Er(XC)$\times 10^3$ & FPR (\%) & FNR (\%) & Time (s) \\
        \hline
        \multicolumn{5}{c}{$p=100$}                                               \\
        21759.63           & 2057.25             & 100.00   & 0.00     & 0.09     \\
        14.58              & 921.75              & 1.86     & 18.70    & 1.34     \\
        18.26              & 1085.43             & 8.04     & 11.76    & 7.41     \\
        10.18              & 695.42              & 3.77     & 13.02    & 8.61     \\
        13.74              & 1106.74             & 64.05    & 0.00     & 9.52     \\
        48.13              & 1574.18             & 30.63    & 9.66     & 21.82    \\
        10.21              & 620.58              & 1.91     & 19.21    & 1.00     \\
        10.47              & 690.08              & 2.44     & 16.18    & 1.07     \\
        12.42              & 721.90              & 2.28     & 15.54    & 0.13     \\
        \hline
        \multicolumn{5}{c}{$p=200$}                                               \\
        99.16              & 2048.96             & 100.00   & 0.00     & 0.11     \\
        8.85               & 1075.74             & 1.26     & 20.12    & 3.97     \\
        7.44               & 1002.65             & 3.68     & 15.97    & 8.74     \\
        6.10               & 783.85              & 2.81     & 13.59    & 9.71     \\
        7.81               & 1405.98             & 81.40    & 0.00     & 13.34    \\
        26.99              & 1163.15             & 33.55    & 7.26     & 25.52    \\
        6.68               & 752.85              & 1.26     & 20.58    & 1.06     \\
        6.92               & 832.53              & 1.61     & 17.57    & 1.08     \\
        7.16               & 786.32              & 1.56     & 16.56    & 0.20     \\
        \hline
        \multicolumn{5}{c}{$p=400$}                                               \\
        67.98              & 2066.17             & 100.00   & 0.00     & 0.44     \\
        5.08               & 1228.47             & 0.76     & 21.34    & 32.78    \\
        4.32               & 1071.54             & 1.97     & 17.34    & 14.06    \\
        3.46               & 897.89              & 1.79     & 14.45    & 13.19    \\
        4.38               & 1721.59             & 64.34    & 0.00     & 39.08    \\
        37.84              & 4856.89             & 31.78    & 17.42    & 12.52    \\
        3.78               & 859.20              & 0.76     & 21.56    & 1.94     \\
        3.96               & 967.03              & 0.96     & 18.20    & 1.71     \\
        4.32               & 948.12              & 0.91     & 17.23    & 0.58     \\
        \hline
        % \multicolumn{6}{c}{Model-1, snr=0.25, r=6}                              \\
      \end{tabular}
    }
  }
  \resizebox{\columnwidth}{!}{
    \subfloat[SNR=0.5, $r=3$]{
    %\subcaptionbox{SNR=0.5, $r=3$}{
      \begin{tabular}{cccccc}
        \hline
        Method            & Er(C)$\times 10^3$ & Er(XC)$\times 10^3$ & FPR (\%) & FNR (\%) & Time (s) \\
        \hline
        \multicolumn{6}{c}{$p=100$}                                                                   \\
        RRR               & 4478.89            & 246.22              & 100.00   & 0.00     & 0.08     \\
        ACS-seq           & 1.34               & 85.83               & 0.96     & 4.54     & 0.50     \\
        ACS-par (rrr)     & 1.54               & 92.22               & 3.24     & 5.92     & 7.00     \\
        ACS-par(lasso)    & 0.97               & 70.50               & 2.10     & 3.56     & 8.08     \\
        SRRR              & 1.66               & 139.64              & 57.32    & 0.00     & 5.28     \\
        SOFAR             & 6.44               & 202.75              & 24.59    & 4.83     & 10.70    \\
        Stage-seq         & 0.65               & 42.58               & 0.85     & 4.52     & 0.38     \\
        Stage-par (lasso) & 0.70               & 52.01               & 1.12     & 3.94     & 1.07     \\
        Stage-par (rrr)   & 0.75               & 46.16               & 1.06     & 3.96     & 0.15     \\
        \hline
        \multicolumn{6}{c}{$p=200$}                                                                   \\
        RRR               & 18.99              & 247.89              & 100.00   & 0.00     & 0.12     \\
        ACS-seq           & 0.78               & 99.79               & 0.67     & 4.46     & 1.68     \\
        ACS-par (rrr)     & 0.77               & 95.32               & 2.03     & 8.71     & 8.08     \\
        ACS-par(lasso)    & 0.55               & 80.38               & 1.58     & 3.33     & 8.84     \\
        SRRR              & 0.85               & 160.50              & 64.31    & 0.00     & 6.98     \\
        SOFAR             & 3.45               & 142.55              & 29.23    & 3.87     & 13.51    \\
        Stage-seq         & 0.41               & 50.72               & 0.59     & 4.12     & 0.47     \\
        Stage-par (lasso) & 0.42               & 61.85               & 0.79     & 3.77     & 1.03     \\
        Stage-par (rrr)   & 0.46               & 54.22               & 0.75     & 3.85     & 0.17     \\
        \hline
        \multicolumn{6}{c}{$p=400$}                                                                   \\
        RRR               & 13.86              & 243.25              & 100.00   & 0.00     & 0.47     \\
        ACS-seq           & 0.46               & 115.37              & 0.44     & 5.17     & 12.47    \\
        ACS-par (rrr)     & 0.46               & 106.39              & 1.22     & 6.40     & 12.83    \\
        ACS-par(lasso)    & 0.31               & 87.26               & 1.13     & 4.12     & 12.41    \\
        SRRR              & 0.49               & 194.07              & 50.02    & 0.00     & 21.94    \\
        SOFAR             & 5.61               & 158.58              & 32.99    & 3.27     & 30.08    \\
        Stage-seq         & 0.24               & 57.48               & 0.37     & 4.87     & 1.03     \\
        Stage-par (lasso) & 0.24               & 67.41               & 0.50     & 4.48     & 1.41     \\
        Stage-par (rrr)   & 0.26               & 61.04               & 0.45     & 4.67     & 0.51     \\
        \hline
        %   \multicolumn{6}{c}{Model-1, snr=0.5, r=3}\\
      \end{tabular}
    }
    \subfloat[SNR=0.5, $r=6$]{
    %\subcaption{SNR=0.5, $r=6$}{
      \begin{tabular}{ccccc}
        \hline
        Er(C)$\times 10^3$ & Er(XC)$\times 10^3$ & FPR (\%) & FNR (\%) & Time (s) \\
        \hline
        \multicolumn{5}{c}{$p=100$}                                               \\
        4788.37            & 478.79              & 100.00   & 0.00     & 0.09     \\
        4.83               & 289.24              & 2.45     & 9.01     & 1.56     \\
        4.71               & 269.37              & 8.38     & 6.11     & 7.45     \\
        6.02               & 402.34              & 4.82     & 6.50     & 8.55     \\
        4.09               & 302.34              & 56.12    & 0.00     & 7.26     \\
        29.85              & 855.91              & 22.83    & 7.75     & 22.13    \\
        3.76               & 215.73              & 2.37     & 10.90    & 0.76     \\
        5.83               & 380.29              & 3.19     & 8.87     & 1.17     \\
        3.57               & 188.62              & 3.17     & 8.03     & 0.13     \\
        \hline
        \multicolumn{5}{c}{$p=200$}                                               \\
        91.45              & 472.36              & 100.00   & 0.00     & 0.11     \\
        2.87               & 340.08              & 1.56     & 10.45    & 5.17     \\
        2.25               & 273.33              & 4.51     & 8.90     & 8.45     \\
        2.42               & 316.90              & 3.58     & 6.79     & 9.50     \\
        1.70               & 287.74              & 65.43    & 0.00     & 14.38    \\
        20.80              & 744.53              & 21.12    & 7.25     & 25.80    \\
        2.25               & 250.90              & 1.53     & 12.55    & 1.01     \\
        2.45               & 306.59              & 2.14     & 9.33     & 1.11     \\
        2.46               & 244.62              & 2.18     & 8.96     & 0.18     \\
        \hline
        \multicolumn{5}{c}{$p=400$}                                               \\
        66.92              & 478.95              & 100.00   & 0.00     & 0.43     \\
        1.80               & 404.84              & 0.92     & 10.43    & 30.04    \\
        1.43               & 306.86              & 2.68     & 9.18     & 14.19    \\
        1.22               & 305.48              & 2.42     & 7.29     & 12.99    \\
        0.99               & 355.65              & 57.26    & 0.00     & 40.66    \\
        29.44              & 554.55              & 26.58    & 7.45     & 10.38    \\
        1.42               & 281.50              & 0.94     & 12.76    & 1.77     \\
        1.57               & 349.37              & 1.36     & 9.97     & 1.66     \\
        1.56               & 278.45              & 1.36     & 9.49     & 0.54     \\
        \hline
        % \multicolumn{6}{c}{Model-1, snr=0.5, r=6}                             \\
      \end{tabular}
    }
  }
\end{table}

\begin{table}
  \caption{Results of Model III under different rank and SNR}\label{tab:model-2}
  \centering
  \resizebox{\columnwidth}{!}{
    \subfloat[SNR=0.25, $r=3$]{
    %\subcaptionbox{SNR=0.25, $r=3$}{
      \begin{tabular}{cccccc}
        \hline
        Method            & Er(C)$\times 10^3$ & Er(XC)$\times 10^3$ & FPR (\%) & FNR (\%) & Time (s) \\
        \hline
        \multicolumn{6}{c}{$p=100$}                                                                   \\
        RRR               & 24652.15           & 1112.40             & 100.00   & 0.00     & 0.09     \\
        ACS-seq           & 3.57               & 255.87              & 0.60     & 0.33     & 0.31     \\
        ACS-par (rrr)     & 7.97               & 484.86              & 8.19     & 2.00     & 7.24     \\
        ACS-par(lasso)    & 3.70               & 258.40              & 1.91     & 0.00     & 8.18     \\
        SRRR              & 7.00               & 574.90              & 63.72    & 0.00     & 6.10     \\
        SOFAR             & 67.08              & 6690.59             & 3.10     & 91.83    & 10.65    \\
        Stage-seq         & 2.26               & 160.14              & 0.51     & 0.31     & 0.45     \\
        Stage-par (lasso) & 3.11               & 217.41              & 1.09     & 0.12     & 1.06     \\
        Stage-par (rrr)   & 3.59               & 242.97              & 1.58     & 0.52     & 0.13     \\
        \hline
        \multicolumn{6}{c}{$p=200$}                                                                   \\
        RRR               & 22.18              & 1123.26             & 100.00   & 0.00     & 0.11     \\
        ACS-seq           & 1.98               & 280.53              & 0.40     & 0.74     & 1.02     \\
        ACS-par (rrr)     & 2.33               & 309.85              & 1.91     & 0.12     & 8.37     \\
        ACS-par(lasso)    & 2.00               & 278.41              & 1.26     & 0.02     & 9.03     \\
        SRRR              & 5.01               & 850.03              & 76.10    & 0.00     & 6.43     \\
        SOFAR             & 36.09              & 7249.85             & 0.20     & 99.50    & 13.44    \\
        Stage-seq         & 1.26               & 176.44              & 0.31     & 0.98     & 0.52     \\
        Stage-par (lasso) & 1.73               & 241.27              & 0.62     & 0.36     & 1.01     \\
        Stage-par (rrr)   & 2.02               & 271.04              & 0.95     & 0.67     & 0.18     \\
        \hline
        \multicolumn{6}{c}{$p=400$}                                                                   \\
        RRR               & 14.25              & 1125.97             & 100.00   & 0.00     & 0.44     \\
        ACS-seq           & 1.18               & 326.43              & 0.20     & 0.79     & 6.63     \\
        ACS-par (rrr)     & 1.29               & 333.69              & 1.06     & 0.26     & 13.02    \\
        ACS-par(lasso)    & 1.14               & 306.51              & 0.77     & 0.07     & 12.81    \\
        SRRR              & 2.62               & 1002.93             & 54.50    & 0.00     & 19.94    \\
        SOFAR             & 18.13              & 7279.39             & 0.00     & 100.00   & 29.29    \\
        Stage-seq         & 0.74               & 201.38              & 0.20     & 0.12     & 1.12     \\
        Stage-par (lasso) & 0.99               & 267.51              & 0.34     & 0.19     & 1.37     \\
        Stage-par (rrr)   & 1.22               & 317.41              & 0.53     & 1.10     & 0.55     \\
        \hline
        % \multicolumn{6}{c}{Model-2, snr=0.25, r=3}                              \\
      \end{tabular}
    }
    \subfloat[SNR=0.25, $r=6$]{
    %\subcaptionbox{SNR=0.25, $r=6$}{
      \begin{tabular}{cccccc}
        \hline
        Er(C)$\times 10^3$ & Er(XC)$\times 10^3$ & FPR (\%) & FNR (\%) & Time (s) \\
        \hline
        \multicolumn{5}{c}{$p=100$}                                               \\
        56647.81           & 2058.84             & 100.00   & 0.00     & 0.09     \\
        10.52              & 714.73              & 1.63     & 3.27     & 0.75     \\
        31.50              & 1648.14             & 22.24    & 8.24     & 7.62     \\
        14.05              & 871.87              & 6.75     & 0.39     & 8.72     \\
        21.68              & 1427.77             & 68.28    & 0.11     & 9.34     \\
        25.09              & 1218.38             & 30.02    & 1.75     & 20.29    \\
        8.00               & 529.77              & 1.73     & 9.76     & 0.97     \\
        14.31              & 885.63              & 4.70     & 9.57     & 1.05     \\
        15.07              & 884.70              & 6.21     & 8.79     & 0.15     \\
        \hline
        \multicolumn{5}{c}{$p=200$}                                               \\
        90.81              & 2085.35             & 100.00   & 0.00     & 0.11     \\
        5.63               & 770.19              & 0.97     & 4.11     & 2.07     \\
        6.90               & 826.20              & 4.99     & 0.01     & 8.52     \\
        7.48               & 903.56              & 4.44     & 0.05     & 9.40     \\
        10.41              & 1539.18             & 83.80    & 0.00     & 9.87     \\
        11.66              & 872.24              & 32.35    & 0.00     & 26.32    \\
        4.18               & 561.83              & 0.88     & 6.42     & 1.18     \\
        7.81               & 953.92              & 2.99     & 9.30     & 1.17     \\
        8.64               & 999.89              & 3.86     & 8.64     & 0.22     \\
        \hline
        \multicolumn{5}{c}{$p=400$}                                               \\
        65.62              & 2051.98             & 100.00   & 0.00     & 0.44     \\
        3.13               & 850.05              & 0.58     & 3.76     & 15.58    \\
        4.53               & 971.92              & 3.66     & 0.25     & 13.36    \\
        4.47               & 1013.68             & 2.98     & 0.06     & 12.87    \\
        5.86               & 1786.83             & 65.21    & 0.00     & 31.25    \\
        22.25              & 1920.62             & 32.38    & 5.11     & 10.11    \\
        2.37               & 623.66              & 0.56     & 8.23     & 1.89     \\
        4.83               & 1120.64             & 1.85     & 10.15    & 1.66     \\
        5.42               & 1177.24             & 2.43     & 8.71     & 0.60     \\
        \hline
        % \multicolumn{6}{c}{Model-2, snr=0.25, r=6}                              \\
      \end{tabular}
    }
  }
  \resizebox{\columnwidth}{!}{
    \subfloat[SNR=0.5, $r=3$]{
    %\subcaptionbox{SNR=0.5, $r=3$}{
      \begin{tabular}{cccccc}
        \hline
        Method            & Er(C)$\times 10^3$ & Er(XC)$\times 10^3$ & FPR (\%) & FNR (\%) & Time (s) \\
        \hline
        \multicolumn{6}{c}{$p=100$}                                                                   \\
        RRR               & 5628.05            & 241.69              & 100.00   & 0.00     & 0.08     \\
        ACS-seq           & 1.15               & 76.76               & 1.07     & 0.31     & 0.38     \\
        ACS-par (rrr)     & 2.05               & 115.89              & 9.37     & 0.64     & 7.05     \\
        ACS-par(lasso)    & 1.17               & 73.86               & 4.12     & 0.00     & 8.11     \\
        SRRR              & 1.86               & 148.12              & 62.70    & 0.00     & 4.82     \\
        SOFAR             & 3.88               & 150.65              & 23.48    & 0.00     & 11.27    \\
        Stage-seq         & 0.64               & 43.43               & 1.23     & 0.57     & 0.35     \\
        Stage-par (lasso) & 0.94               & 61.82               & 2.65     & 0.26     & 1.13     \\
        Stage-par (rrr)   & 0.90               & 57.82               & 3.22     & 1.12     & 0.15     \\
        \hline
        \multicolumn{6}{c}{$p=200$}                                                                   \\
        RRR               & 18.05              & 246.27              & 100.00   & 0.00     & 0.12     \\
        ACS-seq           & 0.62               & 83.42               & 0.73     & 0.62     & 1.15     \\
        ACS-par (rrr)     & 0.62               & 75.61               & 2.81     & 0.00     & 8.25     \\
        ACS-par(lasso)    & 0.64               & 80.90               & 2.87     & 0.00     & 9.02     \\
        SRRR              & 0.98               & 166.66              & 66.31    & 0.00     & 6.54     \\
        SOFAR             & 1.82               & 114.63              & 27.10    & 0.00     & 12.91    \\
        Stage-seq         & 0.36               & 47.35               & 0.67     & 0.67     & 0.43     \\
        Stage-par (lasso) & 0.53               & 66.74               & 1.71     & 1.10     & 0.94     \\
        Stage-par (rrr)   & 0.56               & 67.50               & 2.09     & 0.76     & 0.17     \\
        \hline
        \multicolumn{6}{c}{$p=400$}                                                                   \\
        RRR               & 13.53              & 247.87              & 100.00   & 0.00     & 0.46     \\
        ACS-seq           & 0.35               & 95.23               & 0.40     & 0.33     & 7.20     \\
        ACS-par (rrr)     & 0.37               & 89.29               & 1.89     & 0.00     & 12.65    \\
        ACS-par(lasso)    & 0.37               & 94.57               & 1.73     & 0.00     & 12.67    \\
        SRRR              & 0.58               & 205.47              & 51.19    & 0.00     & 20.32    \\
        SOFAR             & 4.09               & 158.56              & 31.15    & 0.26     & 31.04    \\
        Stage-seq         & 0.20               & 52.19               & 0.36     & 0.67     & 0.96     \\
        Stage-par (lasso) & 0.29               & 75.08               & 0.92     & 0.50     & 1.33     \\
        Stage-par (rrr)   & 0.32               & 75.86               & 1.16     & 0.81     & 0.53     \\
        \hline
      \end{tabular}
    }
    \subfloat[SNR=0.5, $r=6$]{
    %\subcaptionbox{SNR=0.5, $r=6$}{
      \begin{tabular}{ccccc}
        \hline
        Er(C)$\times 10^3$ & Er(XC)$\times 10^3$ & FPR (\%) & FNR (\%) & Time (s) \\
        \hline
        \multicolumn{5}{c}{$p=100$}                                               \\
        10574.61           & 472.34              & 100.00   & 0.00     & 0.08     \\
        5.13               & 334.67              & 2.60     & 1.85     & 0.88     \\
        7.77               & 380.04              & 23.52    & 2.74     & 7.64     \\
        5.36               & 331.75              & 12.05    & 0.27     & 8.61     \\
        5.76               & 365.04              & 66.86    & 0.00     & 6.63     \\
        12.38              & 538.21              & 16.28    & 0.25     & 20.74    \\
        3.87               & 246.22              & 3.42     & 17.39    & 0.88     \\
        5.33               & 336.18              & 8.73     & 5.58     & 1.15     \\
        4.34               & 230.55              & 10.15    & 4.70     & 0.13     \\
        \hline
        \multicolumn{5}{c}{$p=200$}                                               \\
        83.35              & 479.98              & 100.00   & 0.00     & 0.11     \\
        2.87               & 365.76              & 1.72     & 2.81     & 2.64     \\
        2.23               & 224.24              & 8.33     & 0.00     & 8.37     \\
        2.96               & 317.90              & 8.30     & 0.06     & 9.25     \\
        2.42               & 328.58              & 71.09    & 0.00     & 10.14    \\
        5.92               & 401.01              & 15.58    & 0.00     & 27.03    \\
        2.09               & 258.97              & 2.09     & 17.87    & 1.12     \\
        3.00               & 319.34              & 5.64     & 7.87     & 1.17     \\
        2.85               & 272.97              & 6.75     & 5.62     & 0.20     \\
        \hline
        \multicolumn{5}{c}{$p=400$}                                               \\
        64.31              & 478.36              & 100.00   & 0.00     & 0.45     \\
        1.54               & 396.73              & 1.01     & 2.49     & 19.71    \\
        1.54               & 270.46              & 6.17     & 0.00     & 13.25    \\
        1.73               & 337.57              & 5.16     & 0.05     & 12.67    \\
        1.48               & 384.30              & 59.62    & 0.00     & 31.72    \\
        15.87              & 504.32              & 22.85    & 5.14     & 10.49    \\
        1.12               & 276.18              & 1.12     & 15.96    & 1.80     \\
        1.84               & 358.94              & 3.25     & 8.52     & 1.66     \\
        1.87               & 316.16              & 4.02     & 6.83     & 0.59     \\
        \hline
      \end{tabular}
    }
  }
\end{table}

\begin{table}[H]
  \caption{Results of Model-1 and Model-2 under different rank}\label{tab:model-1-2}
  \centering
  \resizebox{\columnwidth}{!}{
    \subfloat[Model-1, $r=3$]{
    %\subcaptionbox{Model-1, $r=3$}{
      \begin{tabular}{cccccc}
        \hline
        Method            & Er(C)$\times 10^3$ & Er(XC)$\times 10^3$ & FPR (\%) & FNR (\%) & Time (s) \\
        \hline
        \multicolumn{6}{c}{$p=100$}                                                                   \\
        RRR               & 783.94             & 60.18               & 100.00   & 0.00     & 0.07     \\
        ACS-seq           & 0.41               & 26.00               & 1.24     & 2.60     & 0.55     \\
        ACS-par (rrr)     & 0.38               & 22.48               & 3.41     & 3.19     & 7.02     \\
        ACS-par(lasso)    & 0.41               & 32.50               & 2.48     & 1.65     & 8.07     \\
        SRRR              & 0.45               & 37.36               & 51.91    & 0.00     & 3.67     \\
        SOFAR             & 2.58               & 79.92               & 16.92    & 3.44     & 11.30    \\
        Stage-seq         & 0.20               & 13.85               & 0.95     & 2.98     & 0.36     \\
        Stage-par (lasso) & 0.43               & 33.35               & 1.20     & 2.48     & 1.09     \\
        Stage-par (rrr)   & 0.22               & 14.65               & 1.21     & 2.71     & 0.12     \\
        \hline
        \multicolumn{6}{c}{$p=200$}                                                                   \\
        RRR               & 18.31              & 59.93               & 100.00   & 0.00     & 0.11     \\
        ACS-seq           & 0.25               & 30.43               & 0.86     & 2.48     & 1.89     \\
        ACS-par (rrr)     & 0.22               & 25.26               & 2.53     & 4.19     & 8.24     \\
        ACS-par(lasso)    & 0.40               & 55.98               & 1.83     & 2.08     & 8.98     \\
        SRRR              & 0.20               & 34.69               & 48.53    & 0.00     & 6.96     \\
        SOFAR             & 2.74               & 87.93               & 18.11    & 3.54     & 12.99    \\
        Stage-seq         & 0.12               & 15.47               & 0.61     & 3.12     & 0.39     \\
        Stage-par (lasso) & 0.45               & 58.98               & 0.82     & 2.33     & 0.94     \\
        Stage-par (rrr)   & 0.13               & 16.33               & 0.80     & 2.75     & 0.14     \\
        \hline
        \multicolumn{6}{c}{$p=400$}                                                                   \\
        RRR               & 13.72              & 59.54               & 100.00   & 0.00     & 0.48     \\
        ACS-seq           & 0.14               & 34.62               & 0.53     & 2.77     & 14.76    \\
        ACS-par (rrr)     & 0.13               & 27.45               & 1.55     & 2.48     & 12.97    \\
        ACS-par(lasso)    & 0.10               & 30.65               & 1.26     & 1.94     & 12.54    \\
        SRRR              & 0.11               & 41.31               & 42.39    & 0.00     & 21.96    \\
        SOFAR             & 5.05               & 75.41               & 24.34    & 3.02     & 28.91    \\
        Stage-seq         & 0.07               & 16.67               & 0.37     & 2.71     & 0.85     \\
        Stage-par (lasso) & 0.10               & 29.02               & 0.51     & 2.31     & 1.31     \\
        Stage-par (rrr)   & 0.08               & 17.16               & 0.48     & 2.42     & 0.48     \\
        \hline
        % \multicolumn{6}{c}{Model-1, snr=1, r=3}                              \\
      \end{tabular}
    }
    \subfloat[Model-1, $r=6$]{
    %\subcaptionbox{Model-1, $r=6$}{
      \begin{tabular}{ccccc}
        \hline
        Er(C)$\times 10^3$ & Er(XC)$\times 10^3$ & FPR (\%) & FNR (\%) & Time (s) \\
        \hline
        \multicolumn{5}{c}{$p=100$}                                               \\
        1316.08            & 117.50              & 100.00   & 0.00     & 0.10     \\
        1.95               & 119.25              & 2.69     & 4.70     & 1.81     \\
        1.17               & 66.79               & 8.61     & 3.16     & 7.55     \\
        8.58               & 507.19              & 5.28     & 3.02     & 8.70     \\
        1.28               & 89.29               & 52.06    & 0.00     & 5.39     \\
        9.05               & 237.90              & 22.17    & 4.68     & 20.43    \\
        1.60               & 93.96               & 2.53     & 7.54     & 0.72     \\
        8.25               & 494.25              & 3.44     & 5.21     & 1.09     \\
        1.43               & 71.81               & 3.62     & 4.68     & 0.10     \\
        \hline
        \multicolumn{5}{c}{$p=200$}                                               \\
        89.91              & 118.99              & 100.00   & 0.00     & 0.11     \\
        1.18               & 137.85              & 1.89     & 5.33     & 5.99     \\
        0.77               & 81.18               & 5.26     & 4.70     & 8.26     \\
        2.80               & 372.96              & 3.98     & 3.84     & 9.20     \\
        0.48               & 72.89               & 43.77    & 0.00     & 14.79    \\
        14.79              & 267.31              & 23.38    & 4.93     & 26.51    \\
        1.19               & 126.18              & 1.73     & 8.90     & 0.83     \\
        3.26               & 412.33              & 2.48     & 6.18     & 1.06     \\
        1.14               & 91.31               & 2.67     & 5.24     & 0.15     \\
        \hline
        \multicolumn{5}{c}{$p=400$}                                               \\
        66.55              & 118.92              & 100.00   & 0.00     & 0.44     \\
        0.76               & 176.14              & 1.13     & 6.18     & 26.40    \\
        0.77               & 98.43               & 3.45     & 4.29     & 14.27    \\
        1.89               & 392.20              & 2.75     & 4.27     & 12.76    \\
        0.24               & 76.96               & 44.47    & 0.00     & 40.29    \\
        28.62              & 254.94              & 25.76    & 5.77     & 10.39    \\
        0.76               & 148.16              & 1.06     & 9.54     & 1.65     \\
        2.18               & 448.83              & 1.70     & 6.85     & 1.71     \\
        1.01               & 130.78              & 1.87     & 6.06     & 0.50     \\
        \hline
        % \multicolumn{6}{c}{Model-1, snr=1, r=6}           \\
      \end{tabular}
    }
  }
  \resizebox{\columnwidth}{!}{
    \subfloat[Model-2, $r=3$]{
    %\subcaptionbox{Model-2, $r=3$}{
      \begin{tabular}{cccccc}
        \hline
        Method            & Er(C)$\times 10^3$ & Er(XC)$\times 10^3$ & FPR (\%) & FNR (\%) & Time (s) \\
        \hline
        \multicolumn{6}{c}{$p=100$}                                                                   \\
        RRR               & 1435.61            & 58.53               & 100.00   & 0.00     & 0.08     \\
        ACS-seq           & 0.45               & 29.22               & 2.11     & 0.00     & 0.45     \\
        ACS-par (rrr)     & 0.50               & 27.56               & 10.20    & 0.05     & 7.07     \\
        ACS-par(lasso)    & 0.38               & 22.94               & 6.72     & 0.00     & 8.00     \\
        SRRR              & 0.56               & 41.43               & 56.04    & 0.00     & 3.75     \\
        SOFAR             & 1.58               & 60.28               & 14.53    & 0.00     & 11.13    \\
        Stage-seq         & 0.24               & 16.56               & 2.20     & 1.86     & 0.36     \\
        Stage-par (lasso) & 0.35               & 24.80               & 4.13     & 0.62     & 1.06     \\
        Stage-par (rrr)   & 0.28               & 18.99               & 4.55     & 1.24     & 0.10     \\
        \hline
        \multicolumn{6}{c}{$p=200$}                                                                   \\
        RRR               & 17.14              & 60.58               & 100.00   & 0.00     & 0.12     \\
        ACS-seq           & 0.27               & 34.42               & 1.44     & 0.00     & 1.40     \\
        ACS-par (rrr)     & 0.19               & 20.71               & 4.63     & 0.00     & 8.05     \\
        ACS-par(lasso)    & 0.22               & 26.05               & 4.69     & 0.00     & 8.76     \\
        SRRR              & 0.24               & 37.62               & 52.25    & 0.00     & 6.59     \\
        SOFAR             & 1.03               & 63.20               & 13.06    & 0.00     & 13.76    \\
        Stage-seq         & 0.14               & 18.50               & 1.36     & 2.83     & 0.39     \\
        Stage-par (lasso) & 0.20               & 27.29               & 2.68     & 0.57     & 0.98     \\
        Stage-par (rrr)   & 0.18               & 22.14               & 3.02     & 0.62     & 0.14     \\
        \hline
        \multicolumn{6}{c}{$p=400$}                                                                   \\
        RRR               & 13.36              & 59.58               & 100.00   & 0.00     & 0.46     \\
        ACS-seq           & 0.14               & 36.68               & 0.74     & 0.00     & 9.36     \\
        ACS-par (rrr)     & 0.11               & 23.05               & 3.25     & 0.00     & 12.69    \\
        ACS-par(lasso)    & 0.12               & 26.31               & 3.12     & 0.00     & 12.30    \\
        SRRR              & 0.13               & 43.79               & 44.63    & 0.00     & 20.71    \\
        SOFAR             & 3.33               & 79.42               & 22.34    & 0.29     & 27.32    \\
        Stage-seq         & 0.08               & 20.27               & 0.67     & 2.17     & 0.83     \\
        Stage-par (lasso) & 0.11               & 27.08               & 1.61     & 1.50     & 1.30     \\
        Stage-par (rrr)   & 0.10               & 24.21               & 1.84     & 1.19     & 0.48     \\
        \hline
      \end{tabular}
    }
    \subfloat[Model-2, $r=6$]{
    %\subcaptionbox{Model-2, $r=6$}{
      \begin{tabular}{ccccc}
        \hline
        Er(C)$\times 10^3$ & Er(XC)$\times 10^3$ & FPR (\%) & FNR (\%) & Time (s) \\
        \hline
        \multicolumn{5}{c}{$p=100$}                                               \\
        2982.15            & 119.12              & 100.00   & 0.00     & 0.10     \\
        3.50               & 218.36              & 4.09     & 2.05     & 1.08     \\
        1.95               & 90.29               & 24.00    & 0.62     & 7.50     \\
        2.42               & 156.27              & 15.91    & 0.12     & 8.53     \\
        2.14               & 120.83              & 60.32    & 0.00     & 4.94     \\
        3.34               & 144.64              & 12.77    & 0.08     & 21.02    \\
        2.55               & 158.18              & 4.71     & 23.98    & 0.83     \\
        2.43               & 158.66              & 11.22    & 6.07     & 1.23     \\
        1.43               & 75.45               & 13.10    & 5.23     & 0.13     \\
        \hline
        \multicolumn{5}{c}{$p=200$}                                               \\
        80.75              & 115.82              & 100.00   & 0.00     & 0.13     \\
        1.84               & 234.30              & 2.65     & 1.67     & 3.37     \\
        0.68               & 60.42               & 12.23    & 0.00     & 8.39     \\
        1.48               & 174.42              & 11.19    & 0.14     & 9.35     \\
        0.71               & 86.00               & 52.32    & 0.00     & 10.20    \\
        2.35               & 143.91              & 13.19    & 0.00     & 27.03    \\
        1.38               & 172.67              & 2.94     & 20.52    & 0.99     \\
        1.52               & 183.12              & 7.27     & 3.24     & 1.17     \\
        0.98               & 86.06               & 8.76     & 3.00     & 0.17     \\
        \hline
        \multicolumn{5}{c}{$p=400$}                                               \\
        64.03              & 118.01              & 100.00   & 0.00     & 0.43     \\
        1.05               & 261.16              & 1.36     & 2.49     & 25.18    \\
        0.61               & 76.78               & 9.07     & 0.00     & 13.39    \\
        0.79               & 138.90              & 7.57     & 0.04     & 12.70    \\
        0.38               & 87.61               & 49.85    & 0.00     & 32.25    \\
        14.56              & 214.41              & 22.41    & 5.10     & 10.42    \\
        0.75               & 176.70              & 1.65     & 23.13    & 1.62     \\
        0.89               & 154.81              & 4.55     & 5.01     & 1.59     \\
        0.84               & 105.73              & 5.61     & 4.44     & 0.54     \\
        \hline
      \end{tabular}
    }
  }
\end{table}
%%% Local Variables:
%%% mode: latex
%%% TeX-master: t
%%% End:
